# Supplementary material for: Mott transition in the A15 phase of Cs$_{3} $C$_{60}$: absence of pseudogap and charge order
Source: arXiv:1610.00513 source file (2017-06-13)
Supplement: Supplementary file 1 [file A15Mott_SuppMat.pdf]

*Supplemental Material*

*for*

# Mott transition in the A15 phase of $Cs_3C_{60}$: absence of pseudogap and charge order

H. Alloul,[1] P. Wzietek,[1] T. Mito,[1] D. Pontiroli,[2]
M. Aramini,[3,2] M. Riccò,[2] J.P. Itie,[4] and E. Elkaim[4]

[1]*Laboratoire de Physique des Solides, CNRS, Univ. Paris-Sud, Université Paris-Saclay, 91405 Orsay, France*

[2]*CNISM and Dipartimento di Fisica, Università di Parma - Via G.P.Usberti 7/a, 43100 Parma, Italy*

[3]*Department of Physics, University of Helsinki, Gustaf Hllstrmin katu 2a, P.O. Box 64 00014 Helsinki, Finland*

[4]*Synchrotron SOLEIL, L'Orme des Merisiers, Saint-Aubin, BP 48, 91192 Gif-sur-Yvette Cedex, France*

(Dated: May 4, 2017)

## I. $^{133}$Cs NMR SPECTRA NEARBY THE MIT

In the paramagnetic states of A15-$Cs_3C_{60}$ the $^{133}$Cs NMR spectra display a quadrupole splitting as the Cs atoms are located on a site in the unit cell which does not have cubic symmetry. The occurrence of the AF phase is detected through the sharp change of linewidth and the shift of the central line which are detected when $T$ is decreased through $T_N = 47$ K (Fig. S1(a)). This is related with the internal field distribution which appears in the AF state [1–3].

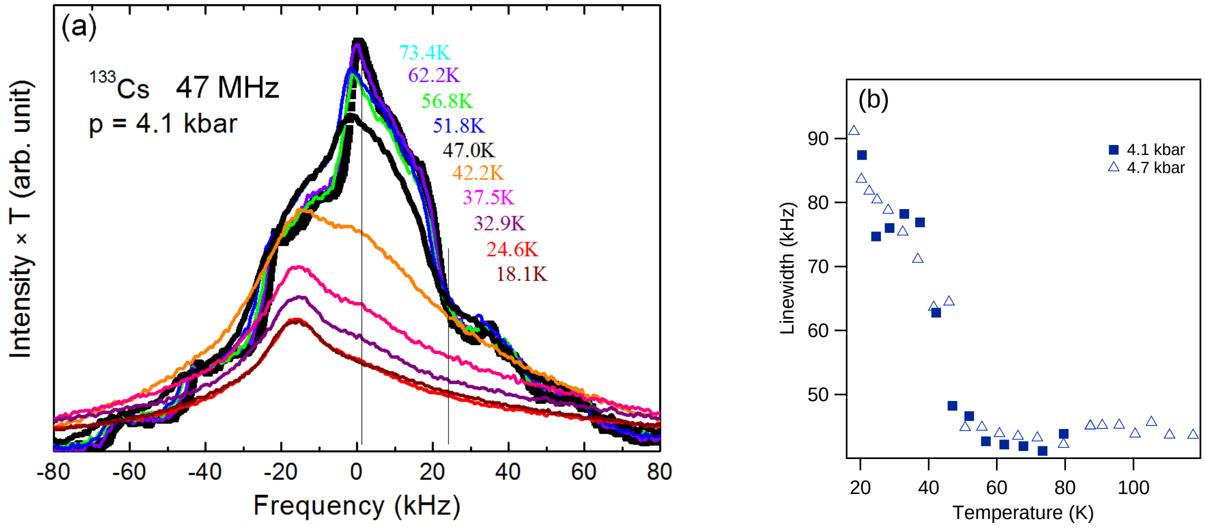


FIG. S1. **(a)** $^{133}$Cs NMR spectra versus $T$ at $p$= 4.1 kbar. There the loss of intensity below $T_N$ is monitored by the spectral intensity in the frequency range delineated near the central $-1/2 \rightarrow 1/2$ transition by two vertical lines. **(b)**: The half intensity linewidth is shown to increase abruptly below $T = 50$ K both for $p =$ 4.1 and 4.7 kbar.

One can also see in Fig. S1(a) that the magnetic broadening in the AF state wipes out already at 42 K all the spectral features linked with the quadrupole satellites. We did not evidence in this Mott insulating phase any significant difference in the $T$ dependence of the $^{133}$Cs NMR spectra between 1 bar and 4.1 kbar, so that $T_N$ is pressure independent within experimental accuracy and the sample remains fully in the Mott state for these pressures as reported in the main text. Below $T_N$ we do monitor in Fig. S1(a) a sizable reduction of the $^{133}$Cs NMR intensity in the range of frequencies delineated there. One might as well characterize the onset of the AF state by reporting the variation of the half intensity NMR linewidth versus $T$, as done in Fig. S1(b). There one can see that one does not detect any difference for 4.1 and 4.7 kbar data, which indicates that $T_N$ remains independent of pressure up to 4.7 kbar.

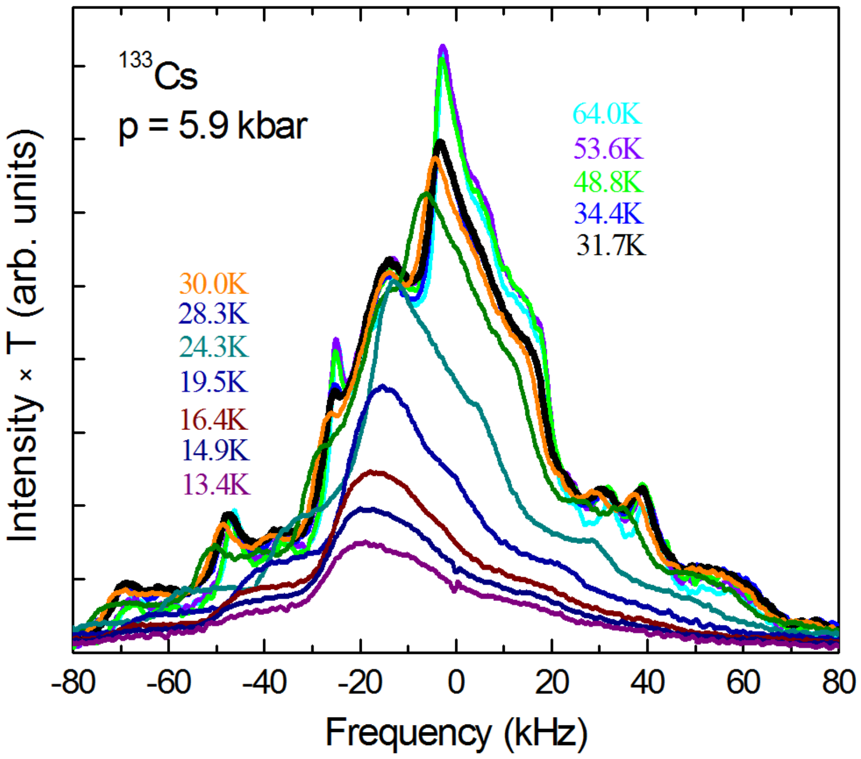


FIG. S2. $^{133}$Cs NMR spectra versus $T$ at $p$= 5.9 kbar. There the signal is unaffected down to the onset of the SC phase at $T_c = 30$ K

At pressures above 5.9 kbar the sample is fully metallic and no modification of the spectrum happens down to $T_c \sim 30$ K as seen in Fig. S2 (and also in ref.[4], Fig.S2)). In the SC state, the penetration of vortices and the associated screening currents induce also a shift and a broadening of the NMR signal. In this case however the quadrupole satellites are still perceptible down to 23 K and in an applied field of 9 Tesla used in these experiments the broadening due to the inhomogeneous field associated with vortices is much smaller than the magnetic broadening in the AF state. In the range of pressures between 4.7kbar and 5.4 kbar we could notice as shown in Fig. S3 that a decrease of intensity in the range of frequencies delineated in Fig. 1(a) is already detectable below 47K. This allowed us to establish the coexistence of AF and SC phases and to estimate the relative fraction of AF phase as explained in Fig. 1 of the main text.

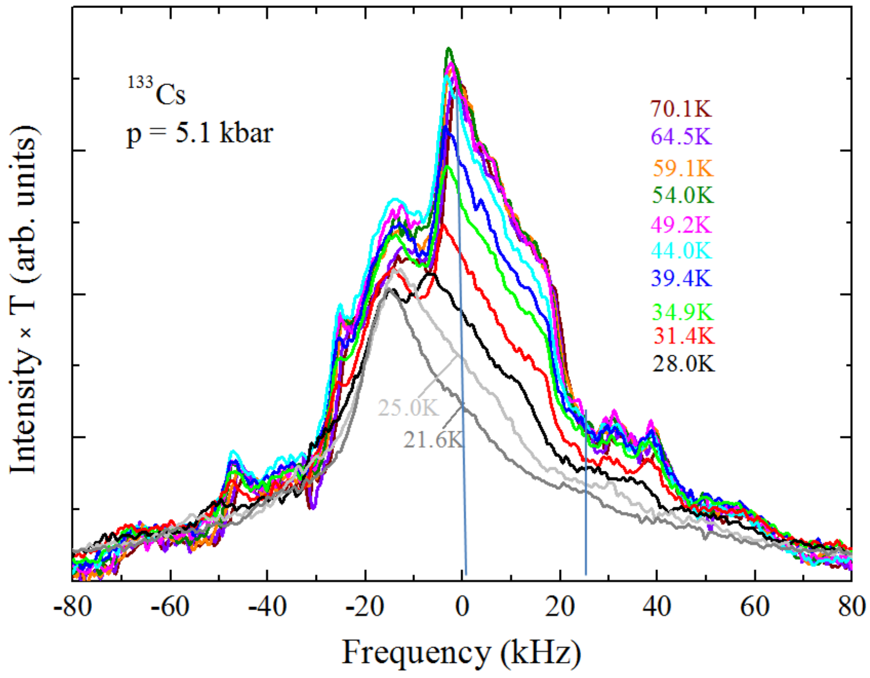


FIG. S3. $^{133}$Cs NMR spectra versus $T$ at 5.1 kbar. Here the loss of intensity associated with the AF component of the signal also onsets at 48K. The quantitative analyses of such data for different pressures are reported in the Fig 1(a) of the main text.

## II. DETAILED FITS OF THE PARAMAGNETIC STATE $^{133}$Cs NMR DATA

We present in Fig. S4 a series of $^{133}$Cs NMR spectra taken at 6.4 kbar in the paramagnetic state of A15-$Cs_3C_{60}$. Those are displayed on a larger frequency range than in Fig S1(a), S2 and S3. One can easily notice there that the spectral shapes exhibit very characteristic quadrupole splittings due to the $I = 7/2$ value of the $^{133}$Cs nuclear spin. Indeed for a single nuclear spin site one expects a spectrum with a central line and six quadrupole satellite lines disposed symmetrically with respect to the central transition. One can see in Fig. S4 that the spectra are quite similar at all temperatures and are only weakly modified at first sight with increasing $T$ though a weak progressive shift of the spectrum is apparent. One cannot evidence easily any obvious sign of the MIT which is located at about 100K from the $T_1$ data of Fig.3 of the main text. Careful fits of the NMR spectra [5] are therefore required to reveal the incidence of the MIT on the $^{133}$Cs spectral parameters. In these spectra the quadrupole frequency ($\nu_Q$ about 40kHz) is much smaller than the Zeeman frequency $\nu_0 = 47$ MHz, so that the former can be treated as a quantum mechanical perturbation [6].

a) *NMR shift*

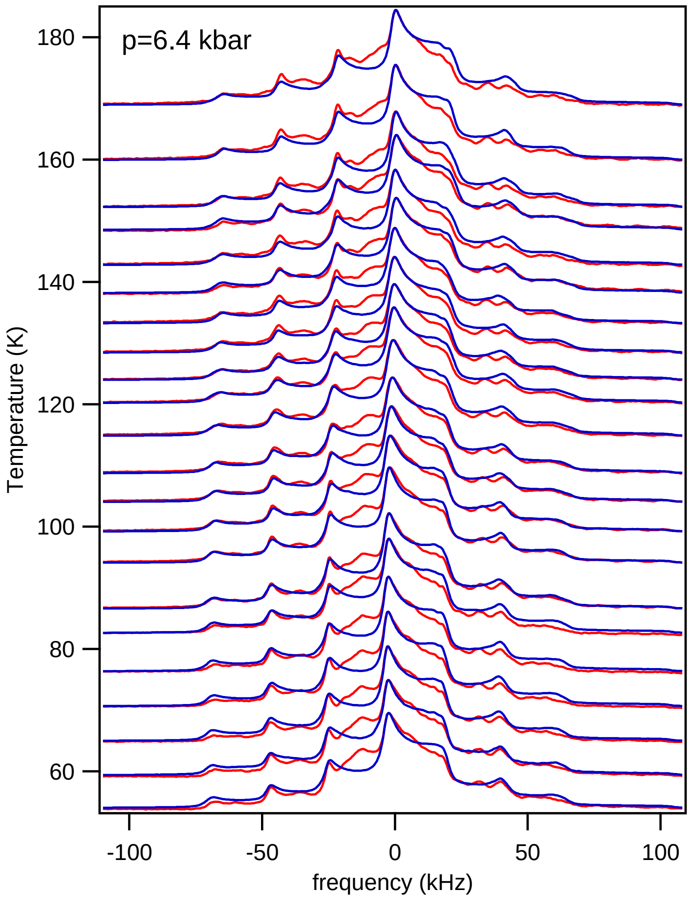


FIG. S4. Series of $^{133}$Cs NMR spectra (in red) taken for $p = 6.4$kbar for distinct $T$ values given on the vertical scale by the position of the baseline of the spectrum. As explained in this supplementary material the (blue) fits of the spectra avoid the range of the $Cs_4C_{60}$ signal which corresponds to the extra contribution seen around -10kHz

.

In Fig. S4 the central transition has clearly a non symetric lineshape which can be assigned to an anisotropic contribution to the NMR shift. Let us notice that the isotropic contribution to the NMR shift is monitored by the position of the central transition. It could be alternatively derived from the first moment of the spectrum as the satellites are symetrical. However in the spectra shown in Fig. S4, a significant unexpected line is seen to occur in all spectra at -10kHz nearby the central transition. This line being present without any symetrical couterpart can hardly be part of the expected single site spin 7/2 nuclear spin spectrum. Knowing the actual existence of distinct $Cs_nC_{60}$ phases, we could easily associate this extra NMR line with that of the spurious

$Cs_4C_{60}$ phase. We did establish that it coincides with the central transition of a phase pure $Cs_4C_{60}$ sample which, being an insulator, displays a lower NMR shift and much longer $T_1$ values. To determine the $^{133}$Cs spectral parameters of the A15 phase we had therefore to avoid giving weight to the signal associated with this spurious $Cs_4C_{60}$ phase. We fitted the spectrum solely in the frequency range outside that of the $Cs_4C_{60}$ signal. The fits were very satisfactory as can be seen in Fig. S4. The anisotropic part $K_{ax}$ of the shift has been found nearly independent of $p$ and $T$ within experimental accuracy, but the isotropic part $K_{iso}$ displays weak $T$ and $p$ dependences which are reported in Fig 3(a) of the main text. This indicates that the two contributions do not have the same physical origin, $K_{ax}$ being for instance orbital or chemical rather than due to spin effects. $K_{iso}$ is found to display a regular increase though the temperature induced metal to insulator transition and shows up a plateau above. This therefore permits us to locate independently the MIT as discussed in the main text.

b) *MIT from NMR shift and* $(T_1T)^{-1}$ *data*

For high $p$ we need to deduce the location of the transition from the various available data. In Fig. S5(a) we present an example of comparison of the $(T_1T)^{-1}$ and $K_{iso}$ data reported in the main text for p=6.4 kbar. These quantities are found to scale perfectly in a large range of temperatures. They only depart from eachother above the temperature of the maximum $T_{max}$ in $(T_1T)^{-1}$ which marks a full restoration of the insulating state. We therefore might think that the metallic range extends up to $T_{max}$. One could as well consider that the transition occurs at the inflexion point of the $(T_1T)^{-1}$ versus $T$ curve. This would correspond to a situation in which $(T_1T)^{-1}$ is a weighted average of the low $T$ metallic behaviour with the high $T$ insulating behaviour associated for instance with an inhomogeneous distribution of pressures in the cell. A heuristic estimation of this temperature $T_{mid(T_1)}$ can be obtained by using a step like function

$$step(T) = 1/2 + atan[(T - T_{mid(T_1)})/\Delta]/\pi$$

with a half intensity width $\Delta$. The data for fixed $p$ are then fitted by

$$(T_1T)^{-1} = (T_1T)_0^{-1} * (1 - step(T)) + (B/(T + \theta)) * step(T) \quad (1)$$

Here the low $T$ metallic behaviour has been taken as a constant $(T_1T)_0^{-1}$ value while the insulating behaviour has been taken as the Curie Weiss like $(T_1T)^{-1} = B/(T + \theta)$. The latter indeed fits quite well the $p = 4.1$ kbar insulator data above 50K as can be sen in Fig. 2(b) in the main text. Such fits for the $(T_1T)^{-1}$ data are shown in Fig. S5(b). In the limited $p$ range explored we

could keep fixed values of $(T_1T)_0^{-1} = 0.2$ s K$^{-1}$ and $B = 15s^{-1}$. We could similarly determine the inflection point $T_{mid(K)}$ of $K_{iso}(T)$ by a similar fit using the function $step(T)$. The deduced values for $T_{mid(T_1)}(p)$, $T_{mid(K)}(p)$ and $\Delta(p)$ have been used in the main text where $T_{max}$, $T_{mid(T_1)}$ and $T_{mid(K)}$ are reported versus $p$ in Fig.4. They give there a good representation of the variation of $T_{MIT}(p)$ in the actual phase diagram, which bends over for increasing $p$ above 5 kbar.

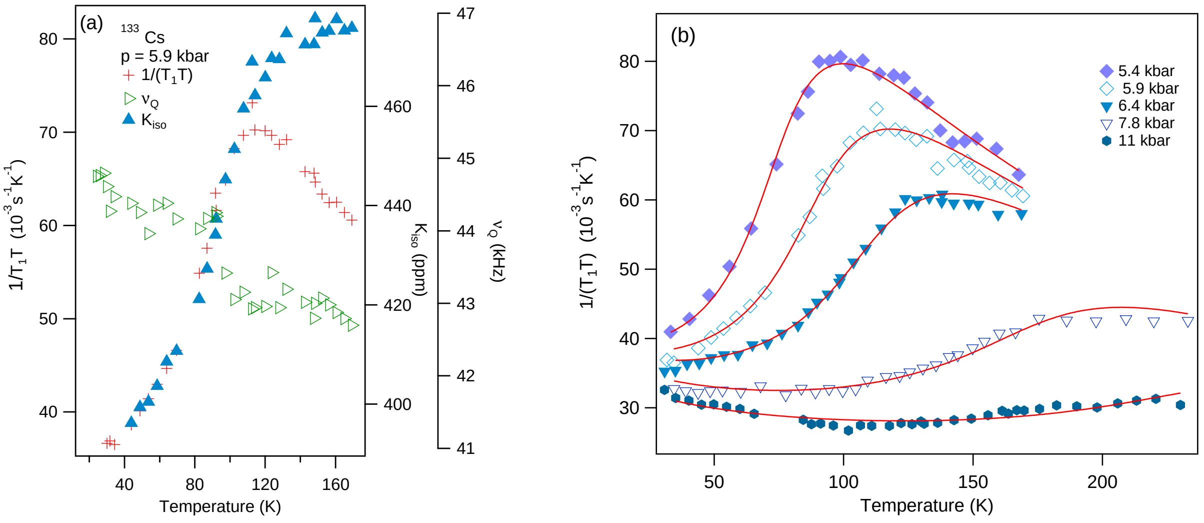


FIG. S5. (a) We report here a comparison of the $T$ dependences of the $(T_1T)^{-1}$ , $K_{iso}$ and $\nu_Q$ data taken at 6.4 kbar. The two former quantities have been scaled to fit eachother in a large range of temperatures surrounding the thermally driven MIT. The $\nu_Q$ transition can be located near the inflexion point of the $(T_1T)^{-1}$ data. (b) The $(T_1T)^{-1}$ data of Fig. 2(b) of the main text can be fitted with Eq. 1 for a large range of pressure values. The data for $T_{max}$ and $T_{mid(T_1)}$ are reported there in Fig. 4 and permit to finalize the phase diagram.

c) *Quadrupole effects in the NMR spectra*

The positions of the qudrupolar satellites of the central NMR line permit estimates of the parameters $\nu_Q$ and $\eta$ which characterize the EFG. The latter is directly connected with the distribution of electric charges around the Cs atoms. From the symmetry of the $^{133}$Cs site in the unit cell of the A15 structure one expects an axial EFG that is $\eta = 0$. But we found that a slightly non zero value is required to reproduce satisfactorily the spectra using a random powder orientation of the EFG axis with respect to the applied magnetic field. We did find that the satellite shapes depend somewhat sensitively on the value taken for $\eta$, and that those seen in the spectra are so sharp that $\eta$ can hardly exceed 0.03. The best fits were obtained with $\eta = 0.02$ and with Euler angles of

(13°,77°, 25°) relating the orientations of the principal axes of the NMR shift and the EFG. One can see that except the signal of the $Cs_4C_{60}$ phase, the simulations fit quite well all other singularities in the spectra. The required non zero $\eta$ value only means that some disorder occurs locally with respect to the ideal symety of the Cs site and results in a distriburion of $\eta$ values which are positive by definition ($\eta = |V_{XX} - V_{YY}|/V_{ZZ}$). This can be due to some orientational disorder of the $C_{60}$ balls. Let us finally point out that the fits are equally good at all temperatures so that this intrinsic disorder is not modified through the MIT. The deduced values of $\nu_Q$ permit us to monitor the evolution of the EFG with $T$ at 6.4 kbar shown in Fig. S5(a) and for a series of fixed $p$ values shown in Fig.3(b) of the main text. The continuous reduction of $\nu_Q$ with increasing $T$ and its small step decrease at the MIT are important measures of the structural variations with increasing $T$ and at the MIT which are discussed in the main text.

d) *Disorder effects evidenced in the quadrupole satellite spectra*

If we examine closely some spectra with a very good signal to noise ratio we do notice some small extra bumps in the signals which are not perfectly fitted with a single site spectrum. One can easily see that those small extra signals occur with similar intensity on both sides of the central line. Overall these spectral contributions might be assigned to a set of low intensity satellites with $\nu_Q$ about 20% smaller than that of the more intense one.

We notice in Fig. S4 that, for $p = 6.4$ kbar, those extra satellites occur in our sample both in the PM state below 50 K and at 150 K in the PI state above the MIT. At 100K they are found as well both at low $p$ in the PI state and at high $p = 11$ kbar in the metalic state as can be seen in Fig. S6. Then these extra signals are not associated with any modification at the Mott transition and are due to intrinsic sample defects. We do consider two possibilities (i) either a structural defect in the A15 phase which could correspond to a static configuration of $C_{60}$ balls with respect to a Cs atom, which reproduces identically on a fraction of Cs sites (about 25% at most).(ii) or that the A15 phase can form in two different isomers distinguished hereagain by the relative orientations of the $C_{60}$ balls.

In the first case there would be an intrinsic disorder of the A15 phase and its macroscopic physical properties would just be sensed by two independent sites. In the second case the two putative phases would appear to have identical physical prperties as we did not detect any singularity on the diamagnetic signal in the SC state. The only differentiation could be within the low $T$ measured "width" of the Mott transition of Fig 1 in the main text. Let us point aout that adding in the Fits of Fig. S4 a second Cs site with 25% intensity and a 20% reduced $\nu_Q$, permits then to fit

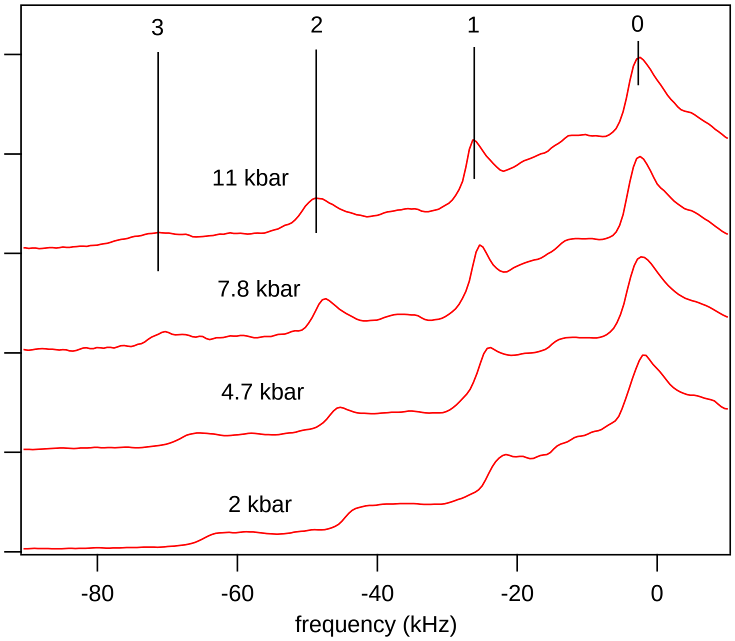


FIG. S6. Spectra taken at $T = 100$ K for selected high $p$ values in the PM state and at low $p$ in the PI state. Here a zoom on the frequency axis has been performed to better visualize the two Cs sites signals. The central line position is pointed out by a vertical line at 0 while the three satellites of the majority Cs sites are located respectively at 1, 2 and 3. One can see the second weak signal peaks with smaller $\nu_Q$ associated with satellites 2 and 3. The large signal between the central line 0 and the first saltellite 1 is associated with the $Cs_4C_{60}$ impurity phase as explained in the fits of Fig. S4.

nearly perfectly the whole NMR spectrum. However the signal to noise ratio is not good enough to permit us reliable determinations of the $p$ and $T$ variations of the parameters which characterize the second site. We cannot therefore ensure whether the $\nu_Q$ and shift values of the two sites track eachother. That would allow to favour (i) or (ii). We shall see in section III below that the XRD data we could take so far are not sufficiently resolved to help to distinguish between (i) and (ii).

## III. X-RAY STRUCTURAL DATA

In-situ powder X-ray diffraction experiment under high pressure was performed on our $Cs_3C_{60}$ samples at the CRISTAL beamline of the synchrotron SOLEIL at the University of Paris-Saclay. During the experiment, three different pressures were explored, respectively 1 bar, 7 kbar and 11 kbar. For the measurement at room pressure, the powdered $Cs_3C_{60}$ (sample AAC1) was put in

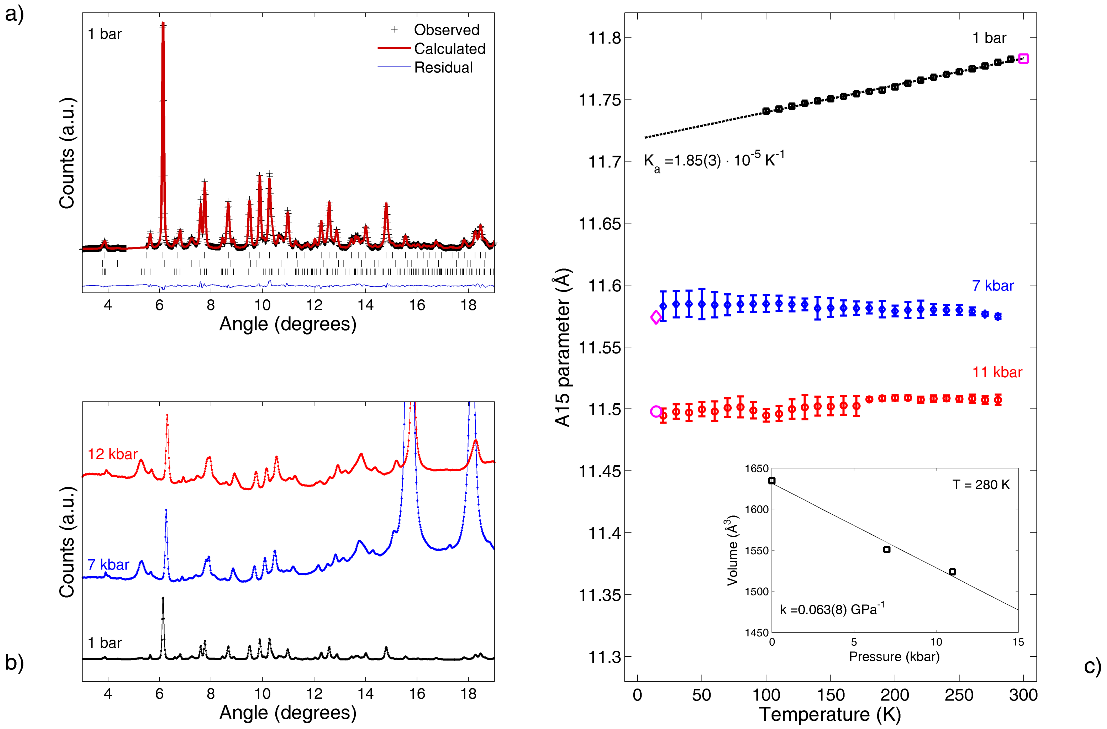


FIG. S7. (a) Rietveld refinement of diffraction data of $Cs_3C_{60}$ collected at 1 bar and 295 K (Rwp = 4%, RF2 = 1.35%). (b) Comparison of powder diffraction patterns collected on the sample at room temperature and different applied pressure. The strong reflections at angles 15.5° and 18° arise from the copper gasket intercepting the x-ray beam. No evident modifications appear in the pressure range 1 bar - 11 kbar. (c) Temperature evolution of the cubic lattice parameter of the A15 phase as a function of temperature for three pressures. Marks in magenta show the data from the literature [8, 9]. Inset: variation of the volume of the A15 cell as a function of the applied pressure at 280 K. The linear fit of the data allowed us to extract the volume compressibility k = 0.063(8) GPa, in good agreement with known data [8].

a glass capillary of 0.7 mm diameter, whereas for the measurements under pressure the sample, previously mixed with Fluorinert®, was placed in a diamond-anvil cell. The loading procedure was performed under Argon atmosphere in a glove box in order to avoid oxygen and moisture contaminations. Possible chemical reactions between $Cs_3C_{60}$ and Fluorinert® were excluded by preliminary X-ray diffraction checks performed at room pressure. After loading, the cell was pressurized and the inner pressure was evaluated by using the ruby fluorescence method [7].

The temperature of the sample was varied in the range 20-300 K by means of a home-built cryostat, operating in $^4$He flux. The diffraction data ($\lambda = 0.56353 \AA$) were collected with a two-dimensional MAR345 detector placed at 20 cm apart from the sample, with typical acquisition time of 10 s. The calibration of the instrument setup was performed using the LaB6 NIST standard reference material 660a. Data manipulation was performed with the Fit2D software, while data treatment was performed with GSAS suite and Matlab. Rietveld refinement of data collected at 1 bar and 295 K, shown in Figure S7-a, confirms the good crystallinity of the sample and allowed us to determine the fractions of the three $Cs_nC_{60}$ phases in the compound, which turn out to be respectively 63.1(1)% A15, 10.0(4)% fcc and 26.9(4)% $Cs_4C_{60}$. On the other hand, typical diffraction patterns collected under pressure show a rather lower S/N ratio, due to the obvious lower amount of sample placed on the beam, slightly broader peaks and the presence of some intense reflections arising from the copper gasket of the diamond-anvil cells, as shown in Figure S7-b. Nevertheless, a reasonable good fit of the data under pressure was obtained as well, by superimposing the diffraction pattern of the three phases, providing that with a different relative amount with respect to the data collected at room pressure, respectively 40% A15, 22% fcc and 38% $Cs_4C_{60}$ for both data taken at 7 and 11 kbar on the same sample. No evident phase-transitions were detected in the investigated temperature and pressure range, as the data were easily fitted only by letting vary the lattice parameters of the three phases, in order to take account of the structural compression induced by the applied pressure, in very good agreement with data present in the literature [8–10]. (NB: the fit with Cs in position 6c is always worse than that with Cs in position 6d, in agreement with literature). The temperature evolution of the cubic lattice parameter in the majority A15 phase was extracted for the three explored pressures by fitting the position of three reflections, respectively (2 1 0), (3 2 0) and (5 2 0), and the results were shown in Figure S7-c. For the data collected at 1 bar, the A15 lattice parameter changes almost linearly with temperature in the range 100-300 K, showing a thermal expansivity of 1.85(3) $10^{-5}$ $K^{-1}$, in good agreement with data taken on the fcc phase [9], as well as on the other fcc $A_3C_{60}$ compounds [11]. On the contrary, under pressure, the lattice parameter variation with $T$ appears strongly reduced. This suggests that the main contribution to the thermal contraction in the fulleride is essentially driven by the "soft" lattice phonons, as expected, rather than any changes in size of the $C_{60}$ molecule. The applied external pressure appears effective in decreasing their anharmonic effects. Finally, although the data taken between 7 kbar and 11 kbar might suggest a slight variation of the lattice parameter in the range 100-200 K, it does fall within the error bars. Small anomalies in the trend might be

depending on uncertainties occurring during the measurement, such as local loss of homogeneity of applied pressure, or small displacements of the sample-holder inside the cryostat.

---


[1] P. Jeglič, D. Arčon, A. Potočnik, A. Y. Ganin, Y. Takabayashi, M. J. Rosseinsky, and K. Prassides, Phys. Rev. B **80**, 195424 (2009).

[2] Y. Ihara, H. Alloul, P. Wzietek, D. Pontiroli, M. Mazzani, and M. Riccó, Europhysics Letters **94**, 37007 (2011).

[3] Y. Ihara, H. Alloul, P. Wzietek, D. Pontiroli, M. Mazzani, and M. Riccò, Phys. Rev. Lett. **104**, 256402 (2010).

[4] P. Wzietek, T. Mito, H. Alloul, D. Pontiroli, M. Aramini, and M. Riccò, Phys. Rev. Lett. **112**, 066401 (2014).

[5] Multi-parameter fits of the NMR spectra were done using the genetic optimisation algorithm described in A. Nelson, J. Appl. Cryst. **39**, 273 (2006).

[6] A. Abragam, *The Principles of Nuclear Magnetism* (Clarendon Press, 1973).

[7] G. J. Piermarini, S. Block, J. D. Barnett, and R. A. Forman, Journal of Applied Physics **46**, 2774 (1975).

[8] A. Y. Ganin, Y. Takabayashi, Y. Z. Khimyak, S. Margadonna, A. Tamai, M. J. Rosseinsky, and K. Prassides, Nature Mat. **7**, 367 (2008).

[9] Y. Takabayashi, A. Y. Ganin, P. Jeglic, D. Arcon, T. Takano, Y. Iwasa, Y. Ohishi, M. Takata, N. Takeshita, K. Prassides, and M. J. Rosseinsky, Science **323**, 1585 (2009).

[10] S. Fujiki, Y. Kubozono, M. Kobayashi, T. Kambe, Y. Rikiishi, S. Kashino, K. Ishii, H. Suematsu, and A. Fujiwara, Phys. Rev. B **65**, 235425 (2002).

[11] G. J. Burkhart and C. Meingast, Phys. Rev. B **54**, R6865 (1996).
